# Supplementary material for: Scenario-Game ADMM: A Parallelized Scenario-Based Solver for Stochastic Noncooperative Games
Source: arXiv:2304.01945 source file (2026-10-09)
Supplement: Supplementary file 1 [file extra_appendix_material.tex]

\newpage

\frank{The following is not relevant to the main paper as of right now:}
~\\

\subsection{Exponential Convergence of Scenario-Game ADMM}

\begin{assumption}\label{assumption: strong monotone assumption}
    The function $F(x;\theta)$ is $m$-strongly-monotone, i.e.,
    \begin{equation}
        (x-y)^\top (F(x;\theta)-F(y;\theta))\ge m\|x-y\|^2,\forall x,y\in \mathbb{R}^n
    \end{equation}
    We assume that the gradient of the function $F(x;\theta)$ and the convex constraint function $h(x;\theta)$ is $L$-Lipschitz continuous.
    % is $L_h$-smooth for all $\theta$, i.e.,
    % \begin{equation}
    %     h(x;\theta)\le h(y;\theta) + \nabla_y h(y;\theta)^\top (x-y) + \frac{L_h}{2} \|x-y\|^2
    % \end{equation}
    Furthermore, we assume that $\|\nabla h(x) + \nabla h(y)\|\le L\|x-y\|_2$. The feasible set $\mathcal{H}:=\{x\in\mathbb{R}^n:h(x;\theta)\le 0\}$ is nonempty and compact.%. In addition, we assume that $\nabla_i h(x;\theta)$ has nonzero singular values for all $x\in \partial \mathcal{H}$ and $i\in[N]$.
\end{assumption}
% {\color{red}Let $H(x;\theta) = [\nabla_i h(x;\theta)]_{i=1}^N$. From the KKT condition of the line 2 of Algorithm~\ref{alg:scenario-admm}, we have
% \begin{equation}
%     \begin{aligned}
%         &\nabla_i f_i (w^j(k+1);\theta^j) + \nabla_i h(w^j(k+1);\theta^j)^\top v_i^* + \lms_i^j(k)\\ & + \rho(w^j(k+1) - Mx_i(k)) = 0\\
%         &v^{*\top} h(w^j(k+1);\theta^j)=0\\
%         &v^*\ge 0,\ \  h(w^j(k+1);\theta^j)\le 0
%     \end{aligned}
% \end{equation}
% }

\begin{lemma}\label{lem: gradient of the Lagrangian is m-strong and L-Lipschitz}
    Under Assumptions~\ref{assumption: ADMM convergence} and \ref{assumption: strong monotone assumption}, let $\{\auxs(k),\vars(k),\lm(k)\}_{k=0}^\infty$ be a sequence of variables returned by Algorithm~\ref{alg:scenario-admm}. In addition, let $\{v^{*}(k)\}_{k=0}^\infty$ be the optimal Lagrange multiplier associated with the inequality constraint in line 2 of Algorithm~\ref{alg:scenario-admm}. Let $\tilde{F}(w^j;\theta^j,v^j):=[\nabla_i f_i(\auxs^j;\params^j)+\nabla_i h(\auxs^j;\params^j)^\top v_{i}^j]_{i=1}^{N}$. Then, $\tilde{F}(\auxs^j;\params^j,v^j)$ is $m$-strongly monotone and $\tilde{L}$-Lipschitz continuous in $\auxs^j$, for some finite $\tilde{L}\in\mathbb{R}$.
\end{lemma}

\begin{theorem}\label{thm:ADMM proof}
    Let the sequences $\{\auxs(k),\vars(k),u(k)\}_{k=1}^\infty$ be generated by Algorithm~\ref{alg:scenario-admm}. Denote by $\auxs^*$, $\vars^*$, $u^*$ the optimal solutions to \eqref{eq:VI optimality condition}. Define $\phi(k):= [\vars(k),u(k)]$ and  $\phi^*:=[\vars^*,u^*]$. Then, for sufficiently large $\kappa_f > (1+v_{max})L/m$, we have
    \begin{equation}\label{eq:upper bound for convergence rate of ADMM}
        \|\phi(k)-\phi^*\|\le  \|\phi(0)-\phi^*\| \Bigg(1-\frac{1}{2 \kappa_f^{0.5+|\epsilon|}}\Bigg)^k,
    \end{equation}
    where $\epsilon = \log_{\kappa_f}(\frac{\mu}{\sqrt{mL}})$.
\end{theorem}

Define $\hat{f}:=\frac{1}{\rho}f$, $\hat{h}:=\frac{1}{\rho}h$ and $\hat{g}:=(\frac{1}{\rho} g)\circ M^\dag + \mathbb{I}_{\textrm{im}\ M}$, where $\mathbb{I}_{\textrm{im} M}$ is the $\{0,\infty\}$-indicator function of the image of $M$. 
% Define $\rho_0:=\rho/\sqrt{mL}$. We have the gradient of $\hat{f}$ is $\rho_0^{-1}\kappa_f^{-0.5}$-strongly monotone and $\rho_0^{-1}\kappa_f^{0.5}$ Lipschitz continuous. 
Finally, we define $s(k):=M\vars(k)$, $u(k) := \frac{\lambda(k)}{\rho}$. Let $\beta(k):= [\nabla_i \hat{f}_i(w_i^j(k);\theta^j)+ \nabla_i h(w_i^j(k+1);\theta^j)^\top v_i^{j*}]_{i=1,j=1}^{N,S}$, where $v_i^{j^*}$ is the optimal dual variable associated with the constraint $h(\auxs^j;\theta)\le 0$.
% \begin{remark}
% \color{red}Check the definition of subdifferential. Make sure we mention that there exists an element in the subgradient set that satisfies the optimality condition.
% \end{remark}
% and $\gamma(k):= [\hat{\eta}_i]_{i=1}^N$, where $\hat{\eta}_i$ is an arbitrary element in $ \partial_i \hat{g}_i(s(k))$.
{\color{red}
\begin{equation}
    \begin{aligned}
        \hat{C}^1 = \begin{bmatrix}
            1+1 & -1+1 \\
            0 & 0
        \end{bmatrix}, \hat{D}^1=\begin{bmatrix}
            -1 & 0 \\
            1 & 0
        \end{bmatrix}
    \end{aligned}
\end{equation}
The construction of this matrix depends on the w and the gradient of f over w.
}

\begin{lemma}[Lyapunov stability]\label{lem:ADMM stability}
    Suppose that $\auxs^*$, $\vars^*$ and $u^*$ are the optimal solution of \eqref{eq:VI optimality condition}. Let $\epsilon = \log_{\kappa_f}(\frac{\mu}{\sqrt{ML}})$ and $\rho_0 = \kappa_f^\epsilon$. Define $\phi(k):= [\vars(k), u(k)]$ and $\phi^*: = [\vars^*, u^*]$. Fix $0< \tau < 1$, and suppose that there exists a positive definite matrix $P\in\mathbb{S}_+^{2SNn}$ and nonnegative constants $\lambda_1,\lambda_2\ge 0$ such that the matrix inequality 
    \begin{equation}\label{eq:stability inequality}
        \begin{aligned}
        &\begin{bmatrix}
            {\color{black}\hat{A}^\top P \hat{A}} - {\color{black}\tau^2 P} & {\color{black}\hat{A}^\top P \hat{B}} \\ {\color{black}\hat{B}^\top P \hat{A}} & {\color{black}\hat{B}^\top P \hat{B}} 
        \end{bmatrix}\\ &+ \begin{bmatrix}
            \hat{C}^1 & \hat{D}^1 \\ \hat{C}^2 & \hat{D}^2 
        \end{bmatrix}^\top \begin{bmatrix}{\color{black}\lambda_1 M_1} & 0 \\ 0 & {\color{black}\lambda_2 M_2} \end{bmatrix} \begin{bmatrix}
            \hat{C}^1 & \hat{D}^1 \\ \hat{C}^2 & \hat{D}^2
        \end{bmatrix} \preceq 0
        \end{aligned}
    \end{equation}
    holds, and the symmetric matrices $M_1$ and $M_2$ are defined by
    \begin{equation}
    \begin{aligned}
        M_1 :=& \begin{bmatrix}
            -2 \rho_0^{-2} & \rho_0^{-1} (\kappa_f^{-\frac{1}{2}} + \kappa_f^{\frac{1}{2}}) & 1 \\ \rho_0^{-1} (\kappa_f^{-\frac{1}{2}} + \kappa_f^{\frac{1}{2}}) & -2 & 0\\ 1 & 0 &0
        \end{bmatrix}\otimes I_{SNn}, \\ M_2:=&\begin{bmatrix}
            0 &1 \\ 1 &1
        \end{bmatrix}\otimes I_{Nn}.
    \end{aligned}
    \end{equation}
    Then, for all $k\ge 0$, we have
    \begin{equation}
        \|\phi(k) - \phi^*\|\le \sqrt{\kappa_P} \|\phi(0) - \phi^*\|\tau^k.
    \end{equation}
\end{lemma}

\begin{proof}
    Let $\auxs^*$, $s^*$, $y^*$, $z^*$ be the optimal values. Define $\beta^* := [\nabla_i \hat{f}_i(\auxs^*)]_{i=1}^N$ and let $\gamma^*\in [\partial_i \hat{g}_i(s^*)]_{i=1}^N$. Multiply \eqref{eq:stability inequality} on the right and its left by $p(k):=[\xi(k) - \xi^*, v(k) - v^*]$ and its transpose, and this leads us to
    \begin{equation}\label{eq:multiplied stability inequality}
        \begin{aligned}
            &p(k)^\top \begin{bmatrix}
            {\color{black}\hat{A}^\top P \hat{A}} - {\color{black}\tau^2 P} & {\color{black}\hat{A}^\top P \hat{B}} \\ {\color{black}\hat{B}^\top P \hat{A}} & {\color{black}\hat{B}^\top P \hat{B}} 
        \end{bmatrix} p(k)\\ &+ p(k)^\top \begin{bmatrix}
            \hat{C}^1 & \hat{D}^1 \\ \hat{C}^2 & \hat{D}^2 
        \end{bmatrix}^\top \begin{bmatrix}{\color{black}\lambda_1 M_1} & 0 \\ 0 & {\color{black}\lambda_2 M_2} \end{bmatrix} \begin{bmatrix}
            \hat{C}^1 & \hat{D}^1 \\ \hat{C}^2 & \hat{D}^2
        \end{bmatrix}p(k) \preceq 0
        \end{aligned}
    \end{equation}
    % Collect the red terms in \eqref{eq:multiplied stability inequality} together, and we can simplify \eqref{eq:multiplied stability inequality} as
    % \begin{equation}\label{eq:expanded stability inequality}
    %     \begin{aligned}
    %         0\ge&{\color{red}\Big(\hat{A}(\xi(k)-\xi^*) + \hat{B}(v(k)-v^*)\Big)^\top P\Big(\hat{A}(\xi(k)-\xi^*) + \hat{B}(v(k)-v^*)\Big)}\\
    %         &-{\color{blue}\tau^2 (\xi(k)-\xi^*)^\top P (\xi(k) - \xi^*)}\\
    %         &+ {\color{orange}\lambda_1\hat{C}^1(\xi(k)-\xi^*) + \hat{D}^1 (v(k)-v^*)^\top M_1\hat{C}^1(\xi(k)-\xi^*) + \hat{D}^1 (v(k)-v^*)}\\
    %         &+ {\color{brown}\lambda_2\hat{C}^2(\xi(k)-\xi^*) + \hat{D}^2 (v(k)-v^*)^\top M_2\hat{C}^2(\xi(k)-\xi^*) + \hat{D}^2 (v(k)-v^*)}
    %     \end{aligned}
    % \end{equation}
    % By Lemma~\ref{lem:ADMM dynamics}, we have
    % \begin{equation}\label{eq:ADMM dynamics with optimal solution}
    %     \begin{aligned}
    %     \begin{bmatrix}
    %         \xi(k+1)-\xi^* \\ y(k)-y^* \\ z(k)-z^*
    %     \end{bmatrix} = \begin{bmatrix}
    %         \hat{A} &  \hat{B} \\ \hat{C} & \hat{D}^1  \\ \hat{C}^2  & \hat{D}^2 
    %     \end{bmatrix}\begin{bmatrix}
    %         \xi(k)-\xi^* \\ v(k)-v^*
    %     \end{bmatrix}.
    %     \end{aligned}
    % \end{equation}
    By Lemma~\ref{lem:ADMM dynamics}, we have
    \begin{equation}
    \begin{aligned}
        0\ge & {\color{black}(\xi(k+1) - \xi^*)^\top P (\xi(k+1) - \xi^*)}\\ & - {\color{black}\tau^2 (\xi(k)-\xi^*)^\top P(\xi(k)-\xi^*)} \\ &+ {\color{black}\lambda_1 (y(k)-y^*)^\top M_1 (y(k)-y^*)}\\ & + {\color{black}\lambda_2(z(k) - z^*)^\top M_2 (z(k) - z^*)}.
    \end{aligned}
    \end{equation}
   % The KKT condition for line 2 of Algorithm~\ref{alg:scenario-admm} is, $\forall i\in[N], \forall j \in[S],$
   %  \begin{equation*}
   %  \begin{aligned}
   %      &\nabla_i f_i (\auxs^j(k+1);\theta^j) + \nabla_i h(\auxs^j(k+1);\theta^j)^\top v_i^{j*} + \lambda_i^j(k)\\ & + \rho(w_i^j(k+1) - x_i(k)) = 0\\
   %      &v_i^{j*\top} h(\auxs^j(k+1);\theta^j)=0,\ 
   %      v_i^{j*}\ge 0,\ \  h(\auxs^j(k+1);\theta^j)\le 0
   %  \end{aligned}
   %  \end{equation*}
   %  where $v^*$ is the optimal dual variable associated with the constraint $h(\auxs^j;\theta^j)\le0$. 
    % 
    Since $\hat{f}$ is $\rho_0^{-1}\kappa_f^{-\frac{1}{2}}$-strongly monotone and $\rho_0^{-1}\kappa_f^{\frac{1}{2}}$-Lipschitz, Lemmas 1~%\ref{lem:IQC for strongly monotone and Lipschitz} 
    and 2 in \cite{nishihara2015general} %~\ref{lem:IQC for convex} 
    imply that the last two terms are non-negative, and therefore, 
    %\dfknote{is there a $k$ missing in the exponent above?}\jingqi{I think in the exponent above, we only consider the relationship between $\xi(k+1)-\xi^*$ and $\xi(k)-\xi^*$. Therefore we don't need to have $k$ in the exponent. }
    \begin{equation}
        (\xi(k) - \xi^*)^\top P (\xi(k) - \xi^*) \le \tau^{2k} (\xi(0)-\xi^*)^\top P (\xi(0) - \xi^*), 
    \end{equation}
    which yields
    \begin{equation}
        \|\xi(k) - \xi^*\|\le \sqrt{\kappa_P} \|\xi(0) - \xi^*\| \tau^k.
    \end{equation}
    Since $\kappa_B=1$, we have
    \begin{equation}
        \|\phi(k) - \phi^*\|\le \sqrt{\kappa_P}\|\phi(0) - \phi^*\|\tau^k.
    \end{equation}
\end{proof}

{\color{red}
\begin{equation}
    v_i^{j}=\left\{\begin{aligned}& 0 &&w_i^j \in \textrm{Int}\ \mathcal{H}\\
        & -\nabla_i h_i(\auxs^j(k+1);\params^j)^\dag (\\&\nabla_i f_i(\auxs^j(k+1);\params^j)+  \\
        & \lm_i^j(k)+\rho (\aux_i^j(k+1)-\var_i(k)) )&& \textrm{otherwise}
    \end{aligned}\right.
\end{equation}

Observe that $\aux_i^{j*}-M\var_i^*=0$
\begin{equation}
    \begin{aligned}
        \|v_i^{j}(k+1) - v_i^{j*} \| \le & L_1 \|\aux_i^j(k+1) - \aux_i^{j*}\| \\
        & L_2 \|\lm_i^j(k+1)-\lm_i^{j*}\|\\
        & L_3 \|x_i^j(k+1)-x_i^{j*}\|
    \end{aligned}
\end{equation}
Can we show
\begin{equation}
    \begin{aligned}
        \|v_i^j(w,x,\lm) - v_i^j(w^*,x^*,\lm^*)\| \le L \left\| \begin{bmatrix}
            w-w^* \\ x-x^* \\ \lm - \lm^*
        \end{bmatrix} \right\|
    \end{aligned}
\end{equation}

}

\begin{proof}[Proof of Lemma~\ref{lem: gradient of the Lagrangian is m-strong and L-Lipschitz}]
    By Theorem~\ref{thm:ADMM convergence}, the sequence $\{\lm(k)\}_{k=0}^\infty$ is bounded. Let $\lambda_{max}: = \max_{k\in\mathbb{Z}_+} \|\lambda(k)\|_{2}$. By KKT condition, Lagrange multipliers are nonzero only if $\vars$ is on the boundary of the feasible set $\mathcal{H}$. Furthermore, we have 
    \begin{equation*}
    \begin{aligned}
        &\nabla_i f(\auxs^j(k+1);\theta) + \nabla_i h(\auxs^j(k+1);\theta)^\top v_i^{j*} \\&+ \lm_i^j(k) + \rho (\aux_i^j(k+1) - \var_i(k))=0
    \end{aligned}
    \end{equation*}
    where $v_i^{j*}$ is the optimal Lagrange multiplier associated with the inequality constraint $h(\auxs;\params^j)\le 0$. In particular, we choose $v_i^{j*}$ such that
    \begin{equation}
        \begin{aligned}
            v_i^{j*} := \min_{v_i^j\ge 0}& \|v_i^j\|_2^2\\
            \textrm{s.t. }&\nabla_i f_i(\auxs^j;\theta^j) + \nabla_i h(\vars;\theta^j)^\top v_i^j\\& + \lm_i^j(k) + \rho(w_i^j(k) -x_i(k))=0\\
            & v_i^{j\top}h(\vars;\theta^j) = 0
        \end{aligned}
    \end{equation}
    Since the feasible set $\mathcal{H}$ is compact and $\lambda(k)$ is upper bounded by $\lm_{\max}$, we can derive an upper bound on $v_i^{j*}$ by
    \begin{equation}
    \begin{aligned}
        v_{max}:=\max_{i\in[N],j\in[S]}\max_{\lambda,x,y,z} \min_{v_i^j\ge 0} & \|v_i^j\|_2^2\\
        \textrm{s.t. }& \nabla_i f_i(x;\theta^j) + \nabla_i h(x;\theta^j)^\top v_i^j\\& + \lambda + \rho(y-z) = 0\\
        & \|\lambda\|_2 \le \lambda_{max}, x,y,z\in \mathcal{H},\\
        & v_i^{j\top}h(x;\theta^j)=0
    \end{aligned}
    \end{equation}
    where $v_{max}$ is finite because $\mathcal{H}$ is compact and there exists an optimal solution to \eqref{eq:VI optimality condition}.
    % For each $\vars\in \partial \mathcal{H}(\theta)$, there exists a set of non-degenerate constraints. Let $\mathcal{I}_i^j$ be the index of coordinate of $h(\auxs^j;\params^j )$. We have a set of non-degenerate constraints $\{h_\ell(\vars;\theta)\}_{\ell\in\mathcal{I}}$. We have
    % \begin{equation}
    %     \nabla_i f(\vars;\theta) + \sum_{\ell\in \mathcal{I}}\nabla_i \tilde{h}_{\ell}(\vars;\theta)^\top \tilde{v}_{i,\ell}^{j*} =         \nabla_i f(\vars;\theta) + \nabla_i h(\vars;\theta)^\top v_i^{j*}
    % \end{equation}
    % Thus, there exists an optimal Lagrange multiplier $\tilde{v}^*\le\sup_{\vars\in \partial \mathcal{H}}\|\nabla \tilde{h}(\vars;\theta)^\dag \|_2(\|F(\vars;\theta)\|_2+\lambda_{max}+2\|\vars\|_2)$.
    % Define the following variables: 
    % \begin{equation*}
    % \begin{aligned}
    %     \lambda_{max}: = \max_{k\in\mathbb{Z}_+} \|\lambda(k)\|_{\infty},F_{max}:=\max_{j\in[S],x\in\partial \mathcal{H}}\|F(x;\theta^j)\|_\infty\\
    %     x_{max}:= \max_{x\in \mathcal{H}}\|x\|_{\infty},\sigma_{min}:=\min_{j\in[S],x\in \partial \mathcal{H}}(\sigma_p(\nabla_x h(x;\theta^j)))
    % \end{aligned}
    % \end{equation*}
    % Let $v_{max}:=\frac{\lambda_{max}+F_{max}+2\rho Nn x_{max}}{\sigma_{min}}$. 
    Since $F(\vars;\theta)$ and $H(\vars;\theta)$ are both $L$-Lipschitz. We have $\tilde{F}(\auxs^j;\theta^j, v^j)$ is $m$-strongly monotone and $(1+v_{max})L$-Lipschitz continuous in $\auxs^j$.
 \end{proof}

\begin{proof}[Proof of Theorem~\ref{thm:ADMM proof}]
    The proof is adapted from \cite{nishihara2015general}. We have it here for completeness. We approach the proof by showing that when $\kappa_f$ is sufficiently large, by taking $\tau = 1- \frac{1}{2}\kappa_f^{-\frac{1}{2}-|\epsilon|}$, $\lambda_1 = \kappa_f^{\epsilon-\frac{1}{2}}$, $\lambda_2=1$, and $P = I_{2SNn}$, the linear matrix inequality \eqref{eq:stability inequality} is satisfied. 
    
    When $\epsilon\ge 0$ and substituting $\tau = 1-\frac{1}{2}\kappa_f^{-\frac{1}{2}-\epsilon}$, the left hand side of \eqref{eq:stability inequality} becomes
    \begin{equation}
        W:=-\frac{1}{4} 
        \kappa_f^{-2} \hat{W}\otimes I_{4SNn}
        % \underbrace{\begin{bmatrix}
        %     \kappa_f^{1-2\epsilon}+4\kappa_f^{\frac{3}{2}-\epsilon} & 8 \kappa_f^{\frac{3}{2}-\epsilon} & 4\kappa_f + 8\kappa_f^{\frac{3}{2}-\epsilon} & 0 \\
        %     8 \kappa_f^{\frac{3}{2}-\epsilon} & 4\kappa_f^2+\kappa_f^{1-2\epsilon} + 4\kappa_f^{\frac{3}{2}-\epsilon} & 4\kappa_f + 4\kappa_f^2 + 8\kappa_f^{\frac{3}{2}-\epsilon} & 0\\
        %     4\kappa_f+8\kappa_f^{\frac{3}{2}-\epsilon} & 4\kappa_f + 4\kappa_f^2 + 8\kappa_f^{\frac{3}{2}-\epsilon} & 8\kappa_f + 4\kappa_f^2 + 8 \kappa_f^{\frac{3}{2}-\epsilon} + 8\kappa_f^{\frac{3}{2}+\epsilon} & 0 \\ 0 & 0 & 0 & 0
        % \end{bmatrix}}_{\hat{M}}.
    \end{equation}
    where $\hat{W}\in \mathbb{R}^{4\times 4}$ is a symmetric matrix and its nonzero entries are defined as $\hat{W}_{11} = \kappa_f^{1-2\epsilon}+4\kappa_f^{\frac{3}{2}-\epsilon}$, $\hat{W}_{12} = 8 \kappa_f^{\frac{3}{2}-\epsilon}$, $\hat{W}_{13} = 4\kappa_f + 8\kappa_f^{\frac{3}{2}-\epsilon}$, $\hat{W}_{22}=4\kappa_f^2+\kappa_f^{1-2\epsilon} + 4\kappa_f^{\frac{3}{2}-\epsilon}$, $\hat{W}_{23}=4\kappa_f + 4\kappa_f^2 + 8\kappa_f^{\frac{3}{2}-\epsilon}$, and $\hat{W}_{33}=8\kappa_f + 4\kappa_f^2 + 8 \kappa_f^{\frac{3}{2}-\epsilon} + 8\kappa_f^{\frac{3}{2}+\epsilon}$. All the other entries of $\hat{W}$ are zeros.

    For sufficiently large $\kappa_f$, the first two leading principle minors of $\hat{W}$ are dominated by $4\kappa_f^{\frac{3}{2}-\epsilon}$ and $16\kappa_f^{\frac{7}{2}-\epsilon}$, respectively. Thus, the first two leading principle minors are positive when $\kappa_f$ is sufficiently large. Subsequently, for sufficiently large $\kappa_f$, when $\epsilon=0$, the third leading principle minor is dominated by $64 \kappa_f^{5}>0$. When $\epsilon>0$, the third leading principle minor is dominated by $128\kappa_f^{5}$. Therefore, for sufficiently large $\kappa_f$, $M$ is a negative semidefinite matrix. Similarly, we can show that when $\epsilon<0$ and substituting $\tau = 1- \frac{1}{2}\kappa_f^{-\frac{1}{2}+\epsilon}$, for sufficiently large $\kappa_f$, the left hand side of \eqref{eq:stability inequality} is still negative semidefinite. By Lemma~\ref{lem:ADMM stability}, we complete the proof.
\end{proof}

\begin{remark}
\color{red}Note that the constriant $Aw-Bx = 0$ or $Ax - Bw = 0$. Possible cases:
\begin{enumerate}
    \item $Aw-Bx= 0$. First parallel unconstrained and then centralized constraint satisfaction. This is ok but cliche.
    \item $Ax - Bw = 0$. First centralized unconstrained and then parallel constraint. But it violates $\hat{f}\circ B^\dag + \mathbb{I}_{\textrm{im\ B}}$ being m-strongly monotone and L-Lipschitz
    \item $Aw-Bx=0$. First parallel constraint and then centralized unconstraint. But it also violates $f(w)$ being m-strongly monotone and L-Lipschitz
\end{enumerate}
\end{remark}

{\color{red}
What if reviewer asks, "what's the relationship between the NE solution in scenario games and the ground truth NE in original game?"
}

{\color{red}
We note here that 
}
